# Supplementary material for: CIPHER: Benchmarking Cross-record Inference over Privacy-Hardened Evidence Records
Source: arXiv:2609.07022 source file (2026-09-07)
Supplement: Supplementary file 1 [file appendix_prompts.tex]

\section{Prompts Details}
\label{sec:appendix_prompts}

\mytcbinput{prompts/CoT.tex}{Chain-of-Thought System Prompt}{0}{bw:domain}{prompt:COT}
\mytcbinput{prompts/FS.tex}{Few-Shot System Prompt}{0}{bw:domain}{prompt:FS}
\mytcbinput{prompts/L2M.tex}{Least-to-Most System Prompt}{0}{bw:domain}{prompt:L2M}
\mytcbinput{prompts/POT.tex}{Program-of-Thought System Prompt}{0}{bw:domain}{prompt:POT}
\mytcbinput{prompts/IE.tex}{FIR Information Extraction Prompt}{0}{bw:domain}{prompt:IE}
\mytcbinput{prompts/JUDGE.tex}{LLM-As-A-Judge Prompt}{0}{bw:domain}{prompt:JUDGE}
